# Supplementary material for: First-principles study on the electronic and optical properties of inorganic perovskite Rb1-xCsxPbI3 for solar cell applications
Source: arXiv:1805.03341 source file (2018-05-09)
Supplement: Supplementary file 1 [file CsRbPbI3-supp.pdf]

# Supporting information – First-principles study on the electronic and optical properties of inorganic perovskite $Rb_{1-x}Cs_xPbI_3$ for solar cell applications

Un-Gi Jong[a,b], Chol-Jun Yu[a]*, Yun-Sim Kim[a], Yun-Hyok Kye[a], and Chol-Ho Kim[b]

[a]*Department of Computational Materials Design, Faculty of Materials Science, Kim Il Sung University, Ryongnam-Dong, Taesong District, Pyongyang, Democratic People's Republic of Korea*

[b]*Natural Science Centre, Kim Il Sung University, Ryongnam-Dong, Taesong District, Pyongyang, Democratic People's Republic of Korea*

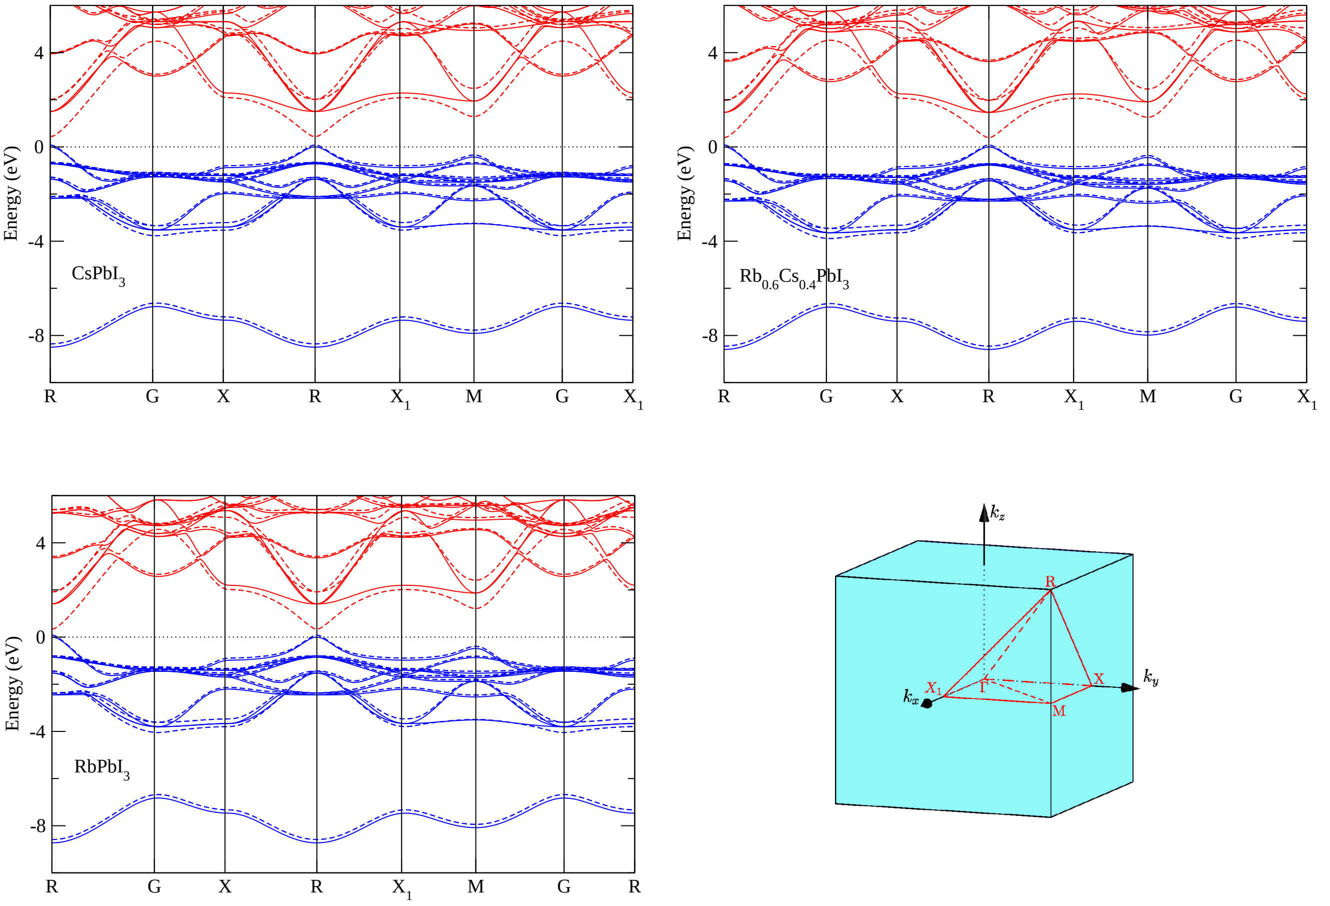


Figure S1. Electronic band structures of $CsPbI_3$, $RbPbI_3$ and $Rb_{0.6}Cs_{0.4}PbI_3$ along the high symmerty *k*-points and lines.

*Corresponding author: Chol-Jun Yu, Email: ryongnam14@yahoo.com

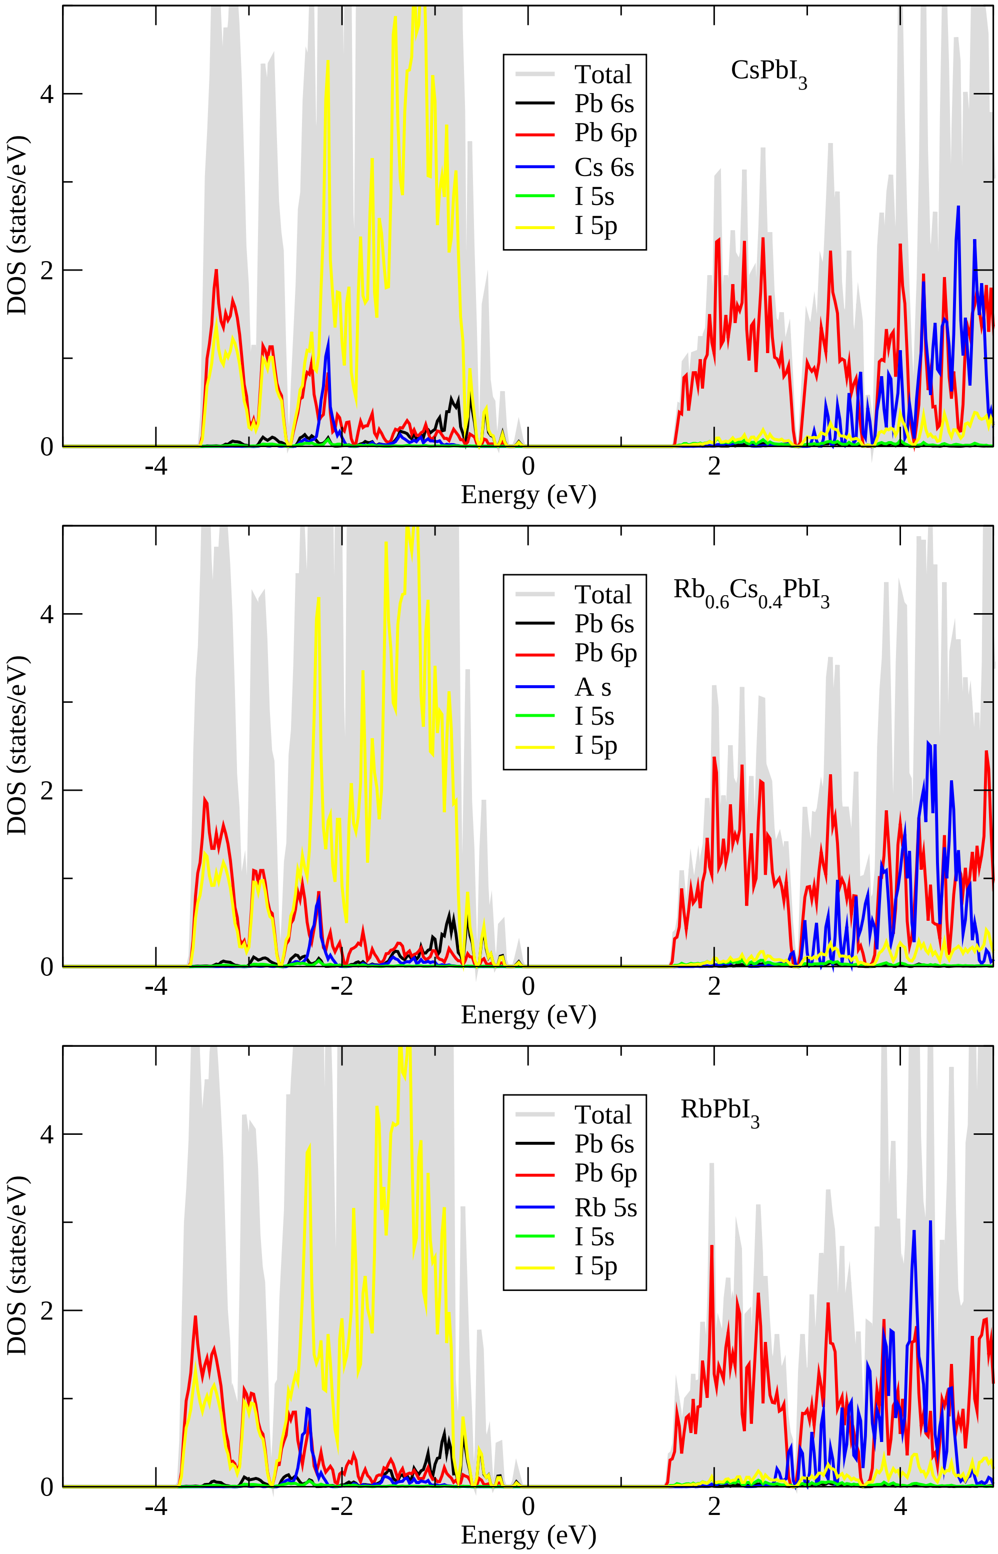


Figure S2. Atomic resolve partial density of states in $CsPbI_3$, $Rb_{0.6}Cs_{0.4}PbI_3$ and $RbPbI_3$.

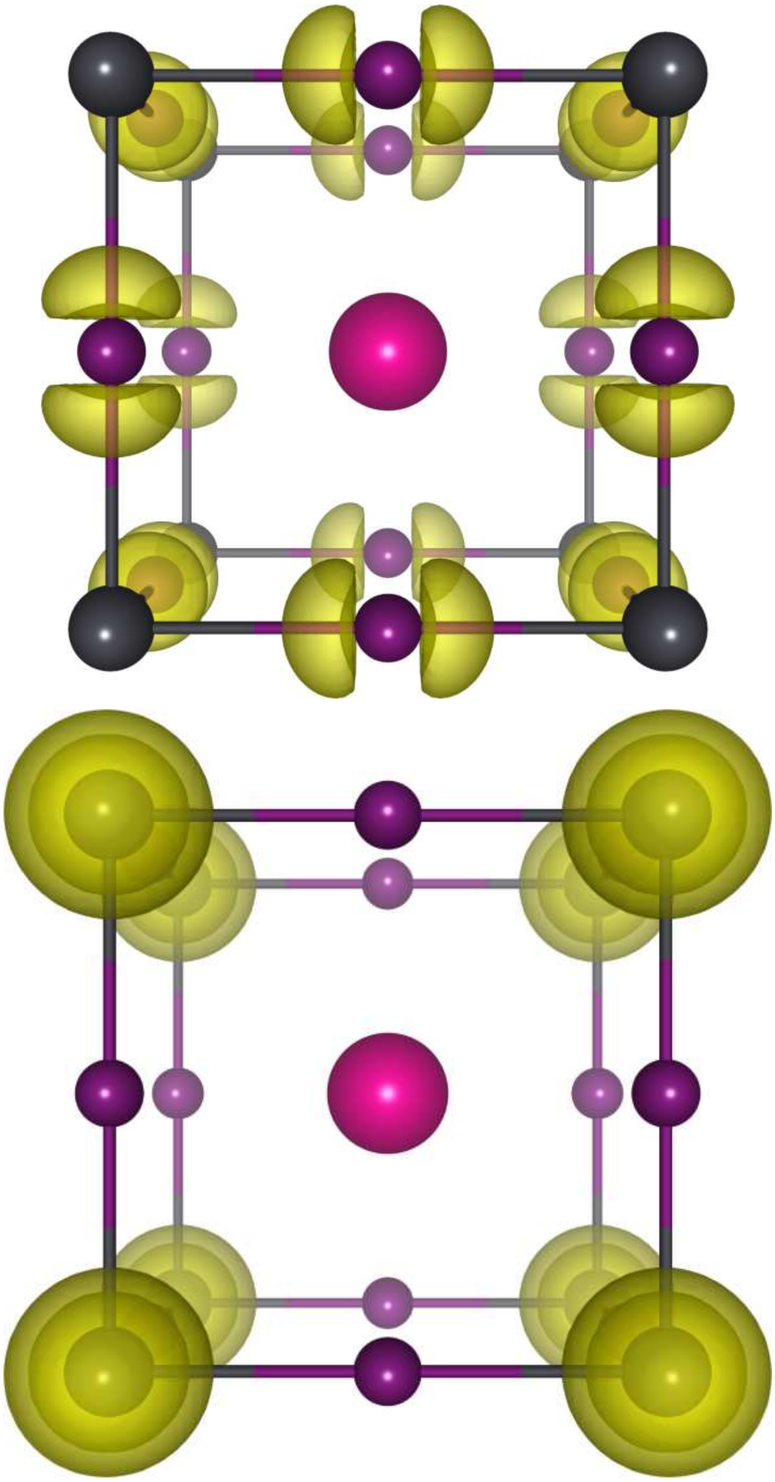

Figure S3. Isosurface plot of the VBM and CBM of $RbPbI_3$.

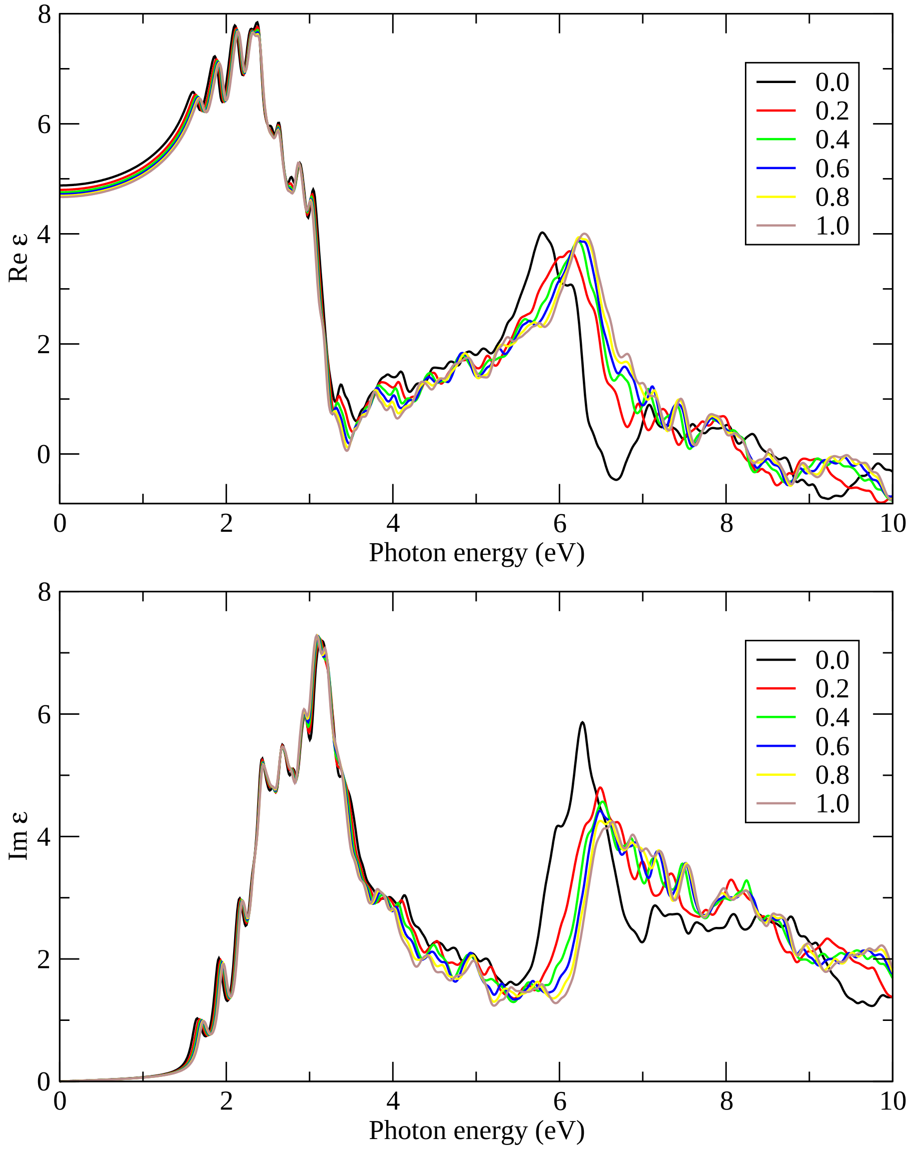


Figure S4. Real and imaginary part of macroscopic dielectric constants as a function of photon energy (frequency) in the inorganic iodide perovskites $Rb_{1-x}Cs_xPbI_3$.
